# Supplementary material for: Nonreciprocal Amplification Transition in a Driven-Dissipative Quantum Network
Source: arXiv:2207.06889 source file (2022-07-14)
Supplement: Supplementary file 1 [file supp.pdf]

# Supplementary Material of "Nonreciprocal Amplification Transition in a Driven-Dissipative Quantum Network"


Mingsheng Tian,[1,*] Fengxiao Sun,[1,*] Kaiye Shi,[2]
Haitan Xu,[3,4,†] Qiongyi He,[1,5,‡] and Wei Zhang[2,6,§]

[1]State Key Laboratory for Mesoscopic Physics, School of Physics, Frontiers Science Center for Nano-optoelectronics, & Collaborative Innovation Center of Quantum Matter, Peking University, Beijing 100871, China
[2]Department of Physics, Renmin University of China, Beijing 100872, China
[3]Shenzhen Institute for Quantum Science and Engineering, Southern University of Science and Technology, Shenzhen 518055, China
[4]School of Physical Sciences, University of Science and Technology of China, Hefei 230026, China
[5]Collaborative Innovation Center of Extreme Optics, Shanxi University, Taiyuan, Shanxi 030006, China
[6]Beijing Academy of Quantum Information Sciences, Beijing 100193, China


* M. Tian and F. Sun contributed equally to this work.


† xuht@sustech.edu.cn

‡ qiongyihe@pku.edu.cn

§ wzhangl@ruc.edu.cn

## I. Derivation of dynamic matrix under periodic boundary condition

By imposing the periodic boundary condition (PBC), the dynamic matrix $M = H + i\Delta\omega\mathbb{I}$ can be rewritten in the plane-wave basis

$$
\begin{aligned}
M_{\mathrm{p}} &= \sum_{j=1}^{N}\sum_{m=0}^{N-1}\mu_m|j+m\rangle\langle j| \\
&= \frac{1}{N}\sum_{j=1}^{N}\sum_{m=0}^{N-1}\mu_m\sum_{k'}e^{-ik'(m+j)}\sum_{k''}e^{ik''j}|k'\rangle\langle k''| \\
&= \frac{1}{N}\sum_{k',k''}\sum_{j=1}^{N}e^{i(k''-k')j}\sum_{m=0}^{N-1}\mu_m e^{-ik'm}|k'\rangle\langle k''| \\
&= \sum_{k}\sum_{m=0}^{N-1}\mu_m e^{-ikm}|k\rangle\langle k| \equiv \sum_{k}h_{\mathrm{p}}(k)|k\rangle\langle k|,
\end{aligned}
\tag{S1}
$$

where we take $|j\rangle = \frac{1}{\sqrt{N}}\sum_{n=0}^{N-1}e^{-ikj}|k\rangle$, and $\delta(k) = \frac{1}{N}\sum_j e^{ikj}$. As $\mu_0 = (\gamma-\kappa-\Gamma)/2 + i\Delta\omega$ and $\mu_{m>0} = -\Gamma e^{-m/\zeta}e^{ik_\omega m}$, we have

$$
h_{\mathrm{p}}(k) = \frac{\gamma-\kappa-\Gamma}{2} + i\Delta\omega - \Gamma\frac{e^{i(k_\omega-k)-1/\zeta} - e^{iN(k_\omega-k)-N/\zeta}}{1-e^{i(k_\omega-k)-1/\zeta}}. \tag{S2}
$$

We can define the winding number as the number of times $h_{\mathrm{p}}(k)$ wrapping around the origin when $k$ increases from $0$ to $2\pi$, and a topological phase transition occurs when the winding number changes.

If the coupling range $\zeta$ is much smaller than the system size $N$ and the detuning $\Delta\omega$ of the input signal is zero, the topological phase transition occurs when

$$
\gamma = \kappa + \Gamma - \frac{2\Gamma}{e^{1/\zeta}+1}. \tag{S3}
$$

By defining the parameter

$$
\xi = \left[\log\left|\frac{\gamma+\Gamma-\kappa+2i\Delta\omega}{\gamma-\Gamma-\kappa+2i\Delta\omega}\right|\right]^{-1},
$$

the phase transition condition can be rewritten as $\zeta = \xi$ provided that the system is in the stable regime with $\gamma < \kappa + \Gamma$. This condition is consistent with the amplification transition condition ($|S_{N1}|^2 = 1$).

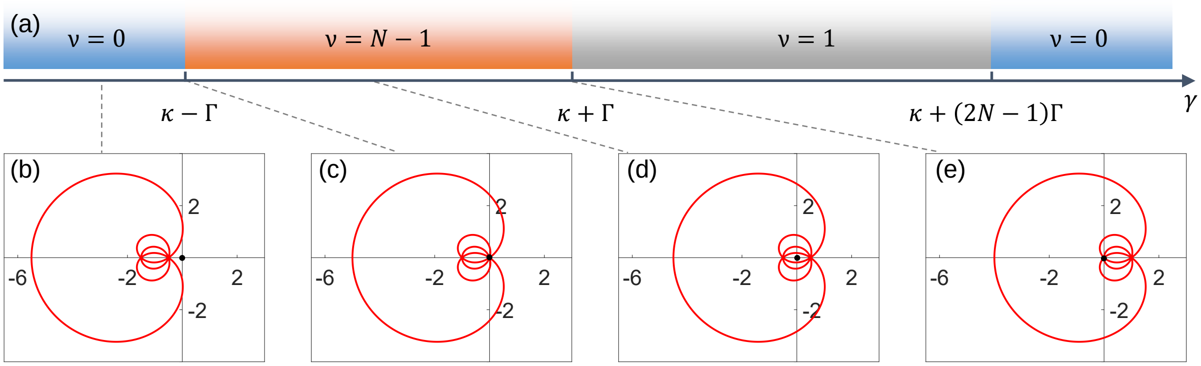


FIG. S1. (a) Phase diagram of the dynamic matrix under the periodic boundary condition. Four different phases can be identified by the winding number $\nu$, and are separated by $\gamma = \kappa - \Gamma$, $\kappa + \Gamma$, and $\kappa + (2N - 1)\Gamma$. (b-e) The complex-energy spectra of $h(k)$ for different pumping rates ($\kappa - 2\Gamma$, $\kappa - \Gamma$, $\kappa$, and $\kappa + \Gamma$, respectively), showing the winding around the origin. In all plots, we take $N = 5$, $\Gamma = 1$, $\Delta\omega = 0$, and $\zeta \gg N$.

However, for the long-range coupling limit ($\zeta \gg N$), the topological phase transition occurs when

$$\gamma = \kappa - \Gamma. \tag{S4}$$

In Fig. S1, we show the phase diagram and the winding behavior of $h_{\rm p}(k)$ in different phases. The topological phase transition condition Eq. (S4) is different from the nonreciprocal amplificaiton transition condition. This observation suggests that one can no longer use the topological phase transition under PBC to predict the transport properties in a system with open boundary condition (OBC).

## II. Edge states for open boundary condition

In the main text, we have defined an auxiliary Hamiltonian by introducing a spin and extending the dynamic matrix to $\mathcal{M}_{\rm o} = M_{\rm o} \otimes \sigma_+ + M_{\rm o}^\dagger \otimes \sigma_-$ with chiral symmetry, where $\sigma_+ = |\uparrow\rangle\langle\downarrow|$ and $\sigma_- = |\downarrow\rangle\langle\uparrow|$ are the spin ladder operators, $|\downarrow\rangle$ and $|\uparrow\rangle$ are the basis states of the auxiliary spin.

Using the singular value decomposition of $M_{\rm o}$ ($M_{\rm o} = U\Lambda V^\dagger$), we have

$$\begin{aligned} \mathcal{M}_{\rm o}(V|\downarrow\rangle + U|\uparrow\rangle) &= (V|\downarrow\rangle + U|\uparrow\rangle)\Lambda, \\ \mathcal{M}_{\rm o}(V|\downarrow\rangle - U|\uparrow\rangle) &= -(V|\downarrow\rangle - U|\uparrow\rangle)\Lambda. \end{aligned} \tag{S5}$$

The columns of $V|\downarrow\rangle \pm U|\uparrow\rangle$ correspond to the eigenvectors. Especially, the $N^{\text{th}}$ column corresponds to the zero-energy edge states .

The auxiliary Hamiltonian $\mathcal{M}_{\text{o}}$ has the form

$$\mathcal{M}_{\text{o}} = \sum_{m=0}^{N-1}\sum_{j=1}^{N-m} \mu_m \,|j+m,\uparrow\rangle\langle j,\downarrow| + \sum_{m=0}^{N-1}\sum_{j=1}^{N-m} \mu_m \,|j,\downarrow\rangle\langle j+m,\uparrow| \,. \tag{S6}$$

The zero-energy eigenstates of this Hamiltonian satisfy

$$\mathcal{M}_{\text{o}} \sum_{n=1}^{N} (a_n|n,\downarrow\rangle + b_n|n,\uparrow\rangle) = 0. \tag{S7}$$

This gives $2N$ equations for the amplitudes $a_n$ and $b_n$ as follows,

$$\begin{aligned} \text{for } n = 2, 3..., N-1: \qquad & \textstyle\sum_{m=1}^{n} a_m \mu_{n-m} = 0; \quad \sum_{m=n}^{N} b_n \mu^*_{m-n} = 0; \\ \text{for boundaries}: \qquad & a_1\mu_0 = 0; \qquad b_N\mu_0^* = 0; \end{aligned} \tag{S8}$$

Note that $\mu_j = \mu_k c^{j-k}$ with $c = e^{-1/\zeta}$ for all $j, k > 0$.

The solution to the above equations is

$$\begin{aligned} a_n &= a_N\left(c - \frac{\mu_1}{\mu_0}\right)^{-(N-n)}, \quad \text{for } n = 2\ldots, N; \qquad a_1 = -a_N\frac{\mu_0}{\mu_1}\left(c - \frac{\mu_1}{\mu_0}\right)^{-(N-2)}; \\ b_n &= b_1\left(c^* - \frac{\mu_1^*}{\mu_0^*}\right)^{-(n-1)}, \quad \text{for } n = 1, \ldots, N-1; \quad b_N = -b_1\frac{\mu_0^*}{\mu_1^*}\left(c^* - \frac{\mu_1^*}{\mu_0^*}\right)^{-(N-2)}. \end{aligned} \tag{S9}$$

If $|c - \mu_1/\mu_0| > 1$, by defining the localization length

$$\xi' = \frac{1}{\log|\mathrm{c} - \mu_1/\mu_0|}, \tag{S10}$$

Eq. (S9) can be rewritten as

$$\begin{aligned} |a_n| &= |a_N|e^{-(N-n)/\xi'}, \quad \text{for } n = 2, \ldots, N; \qquad |a_1| = \left|a_N\frac{\mu_0}{\mu_1}\right| e^{-(N-2)/\xi'}; \\ |b_n| &= |b_1|e^{-(n-1)/\xi'}, \quad \text{for } n = 1, \ldots, N-1; \quad |b_N| = \left|b_1\frac{\mu_0^*}{\mu_1^*}\right| e^{-(N-2)/\xi'}; \end{aligned} \tag{S11}$$

where $|a_N| = |b_1| = \left|\frac{c\mu_0 - \mu_0 - \mu_1}{c\mu_0 - \mu_1}\right|$. Thus, in the thermodynamic limit ($N \to \infty$), we have two

zero-energy solutions,

$$|L\rangle = \sum_{n=1}^{N} a_n |n, \downarrow\rangle, \quad |R\rangle = \sum_{n=1}^{N} b_n |n, \uparrow\rangle. \tag{S12}$$

The exponentially small coupling between the two states $|L\rangle$ and $|R\rangle$ induces an exponentially small energy splitting. We can estimate the splitting and the resulting eigenenergies to a good approximation using adiabatic elimination of the other eigenstates [1]. In this approximation, the central quantity is the overlap

$$|\langle R|\mathcal{M}_{\mathrm{o}}|L\rangle| = a_1 b_1 \mu_0 = \left| \frac{{\mu_0}^2}{\mu_1} a_N b_1 e^{-(N-2)/\xi'} \right|. \tag{S13}$$

Thus the eigenstates and eigenvalues are approximated as

$$|0\pm\rangle = \frac{|L\rangle \pm |R\rangle}{\sqrt{2}}, \quad \lambda_\pm = \pm |a_1 b_1 \mu_0| = \pm \left| \frac{{\mu_0}^2}{\mu_1} a_N b_1 e^{-(N-2)/\xi'} \right|; \tag{S14}$$

The energies of the hybridized states are exponentially small with increasing system size.

In our model, as the zero-energy edge state corresponds to the $N^{\mathrm{th}}$ column of $V|\downarrow\rangle + U|\uparrow\rangle$, we have $|V_{jN}| = |a_j| = N_0 e^{-(N-j)/\xi'}$ and $|U_{lN}| = |b_l| = N_0 e^{-(l-1)/\xi'}$, where $N_0 = |a_N| = |b_1|$. Especially, by taking $\mu_0 = (\gamma - \kappa - \Gamma)/2$, $\mu_1 = -\Gamma c$, $c = e^{-1/\zeta + ik_\omega}$, $\xi = 1/\log\left|\frac{\gamma+\Gamma-\kappa}{\gamma-\Gamma-\kappa}\right|$ and considering the stable condition $\gamma < \kappa + \Gamma$, we can rewrite the above results as in the main text. The normalization parameter $N_0$ becomes

$$N_0 = \left| 1 - \frac{e^{1/\zeta - \mathrm{i}k_\omega}(\gamma - \Gamma - \kappa)}{\gamma + \Gamma - \kappa} \right|. \tag{S15}$$

The eigenvalues in Eq. (S14) become

$$\lambda_\pm = \pm \frac{e^{-1/\zeta}(\gamma + \Gamma - \kappa)^2}{4\Gamma} N_0^2 e^{-N/\xi'}. \tag{S16}$$

The localization length of edge state in Eq. (S10) becomes

$$\xi' = 1/\log \left| \frac{e^{-1/\zeta}(\gamma + \Gamma - \kappa)}{\gamma - \Gamma - \kappa} \right| = \frac{1}{\xi^{-1} - \zeta^{-1}}. \tag{S17}$$

The condition $\xi' > 0$ can be rewritten as $\zeta > \xi$, which is consistent with the nonreciprocal

amplification condition ($|S_{N1}|^2 = 1$) as given by Eq. (3) in the main text.

[1] J. K. Asbóth, L. Oroszlány, and A. Pályi, “A short course on topological insulators,” (Springer, New York, 2016) Chap. 1, pp. 1–20.
